# Supplementary material for: SPEC: Seeing People in the Wild with an Estimated Camera
Source: arXiv:2110.00620 source file (2022-11-01)
Supplement: Supplementary file 1 [file supmat_agora.tex]

\begin{table}
    \centering
    \resizebox{0.47\textwidth}{!}{
        \begin{tabular}{l|r|r|r|r|r}
        \toprule
        \textbf{Methods} & \textbf{\mpjpe} & \textbf{\wmpjpe} & \textbf{\pampjpe} & \textbf{\wpve} & \textbf{\pve}\\ 
        \midrule 
        GraphCMR~\cite{kolotouros2019cmr} & 195.6 & 198.3 / 197.2 & 71.6 & 215.1 / 227.9 & 216.8 \\
        SPIN~\cite{SPIN:ICCV:2019} & 171.0 & 178.9 / 172.7 & 72.5 & 194.8 / 200.9 & 185.8 \\
        % Pose2Mesh~\cite{Choi_2020_ECCV_Pose2Mesh} & & & & & \\
        PartialHumans~\cite{Rockwell2020} & 189.8 & 187.5 / 191.3 & 82.2 & 202.6 / 220.7 & 209.0 \\
        I2L-MeshNet$^{\dagger}$~\cite{Moon_2020_ECCV_I2L-MeshNet} & 171.6 & 180.8 / 173.2 & 71.6 & 195.9 / 203.2 & 194.4 \\
        % CenterHMR~\cite{CenterHMR} & 185.5 & 70.3 & 197.4 \\
        % CRMH~\cite{jiang2020mpshape} & & & & & \\ 
        \midrule
        HMR$^{*}$~\cite{kanazawa_hmr} & 90.0 & 132.7 / 100.0 & 50.7 & 144.2 / 111.5 & 102.0 \\
        \methodname & \textbf{77.9} & \textbf{79.1} /\textbf{79.1} & \textbf{49.8} & \textbf{94.0} / \textbf{94.0} & \textbf{92.2} \\
        \bottomrule
        \end{tabular} 
    }
    \caption{Results of SOTA methods on \agoracam. See Table~\ref{tab:sota_mtp} caption.
    }
    \vspace{-1ex}
    \label{tab:sota_agora}
\end{table}
