# Supplementary material for: SPEC: Seeing People in the Wild with an Estimated Camera
Source: arXiv:2110.00620 source file (2022-11-01)
Supplement: Supplementary file 3 [file supmat_smplify_agora.tex]

\begin{table}[]
    \centering
    \resizebox{0.48\textwidth}{!}{
        \begin{tabular}{l|r|r|r}
        \toprule
        \textbf{Methods} & \textbf{\wmpjpe} & \textbf{\pampjpe} & \textbf{\wpve} \\ \midrule
        SMPLify-X (ground-truth $f$) & 138.5 / 119.9 & 67.6 & 151.5 / 133.4 \\ 
        \midrule
        SMPLify-X \cite{SMPL-X:2019} ($f=5000$) & 179.3 / 159.8 & 71.6 & 191.5 / 191.0 \\ 
        SMPLify-X \cite{kissosECCVW2020} ($f=2200$) & 164.2 / 141.8 & 70.1 & 176.9 / 155.3 \\ 
        \midrule
        SMPLify-X (\camcalib $K$) & 143.3 / 122.2 & \textbf{67.4} & 156.3 / 135.8 \\
        \smplify (\camcalib $K$ + $\camrot$) & \textbf{121.9} / \textbf{121.9} & 67.8 & \textbf{135.0} / \textbf{135.0} \\ 
        \bottomrule
        \end{tabular} 
    }
    \caption{{\bf HPS optimization with an estimated camera.}  \smplify on the \agoracam dataset.}
    \label{tab:smplify_agora}
\end{table}
